# Supplementary material for: DepthP+P: Metric Accurate Monocular Depth Estimation using Planar and Parallax
Source: arXiv:2301.02092 source file (2023-01-05)
Supplement: Supplementary file 3 [file pp.tex]

\begin{figure*}[t]
    \includegraphics[width=0.49\linewidth]{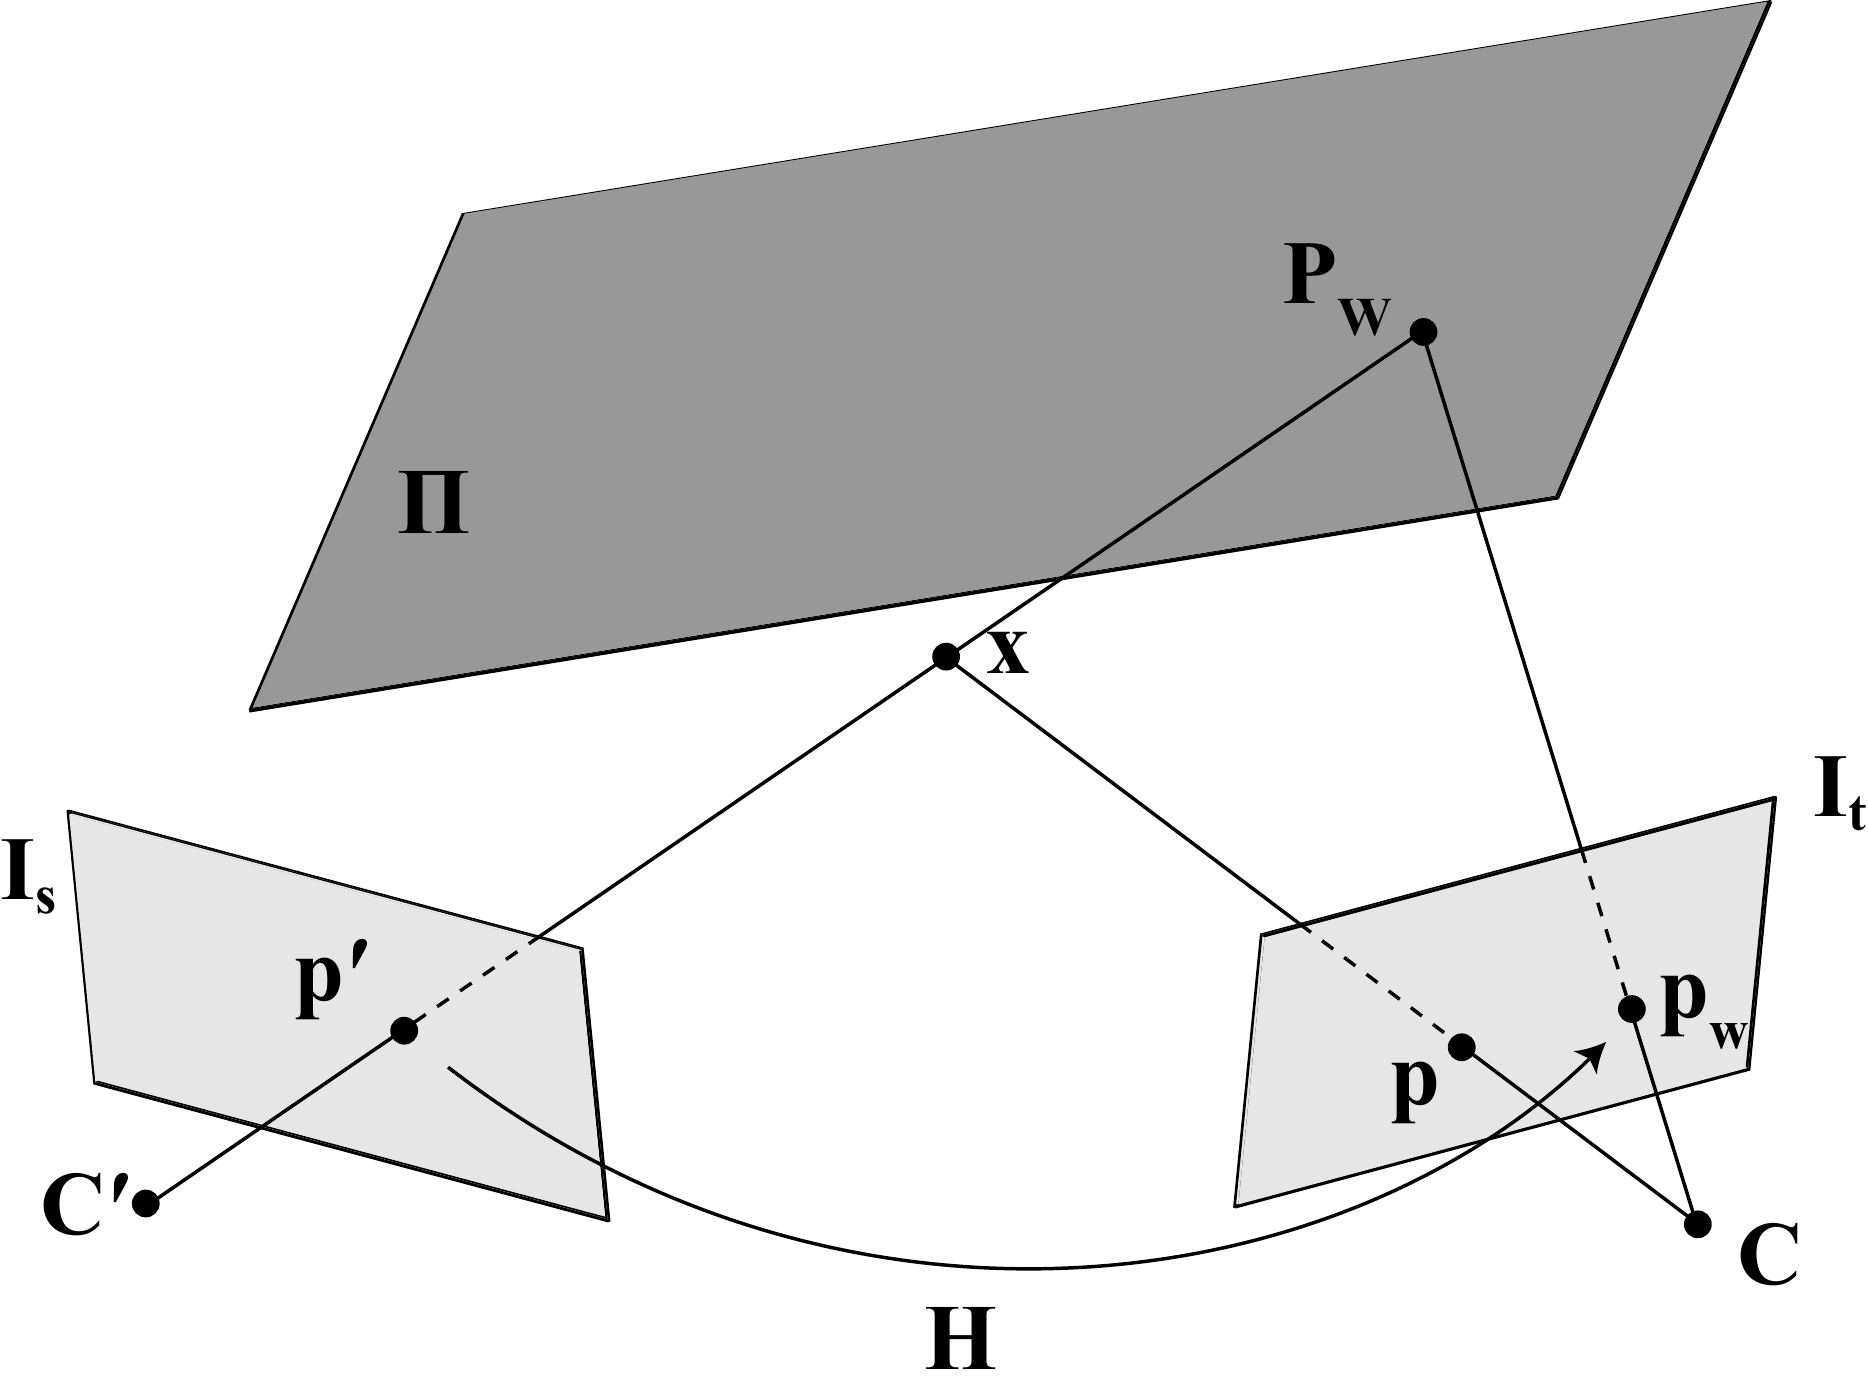}
    \hspace{0.02\linewidth}
    \raisebox{0.7cm}{\includegraphics[width=0.49\linewidth]{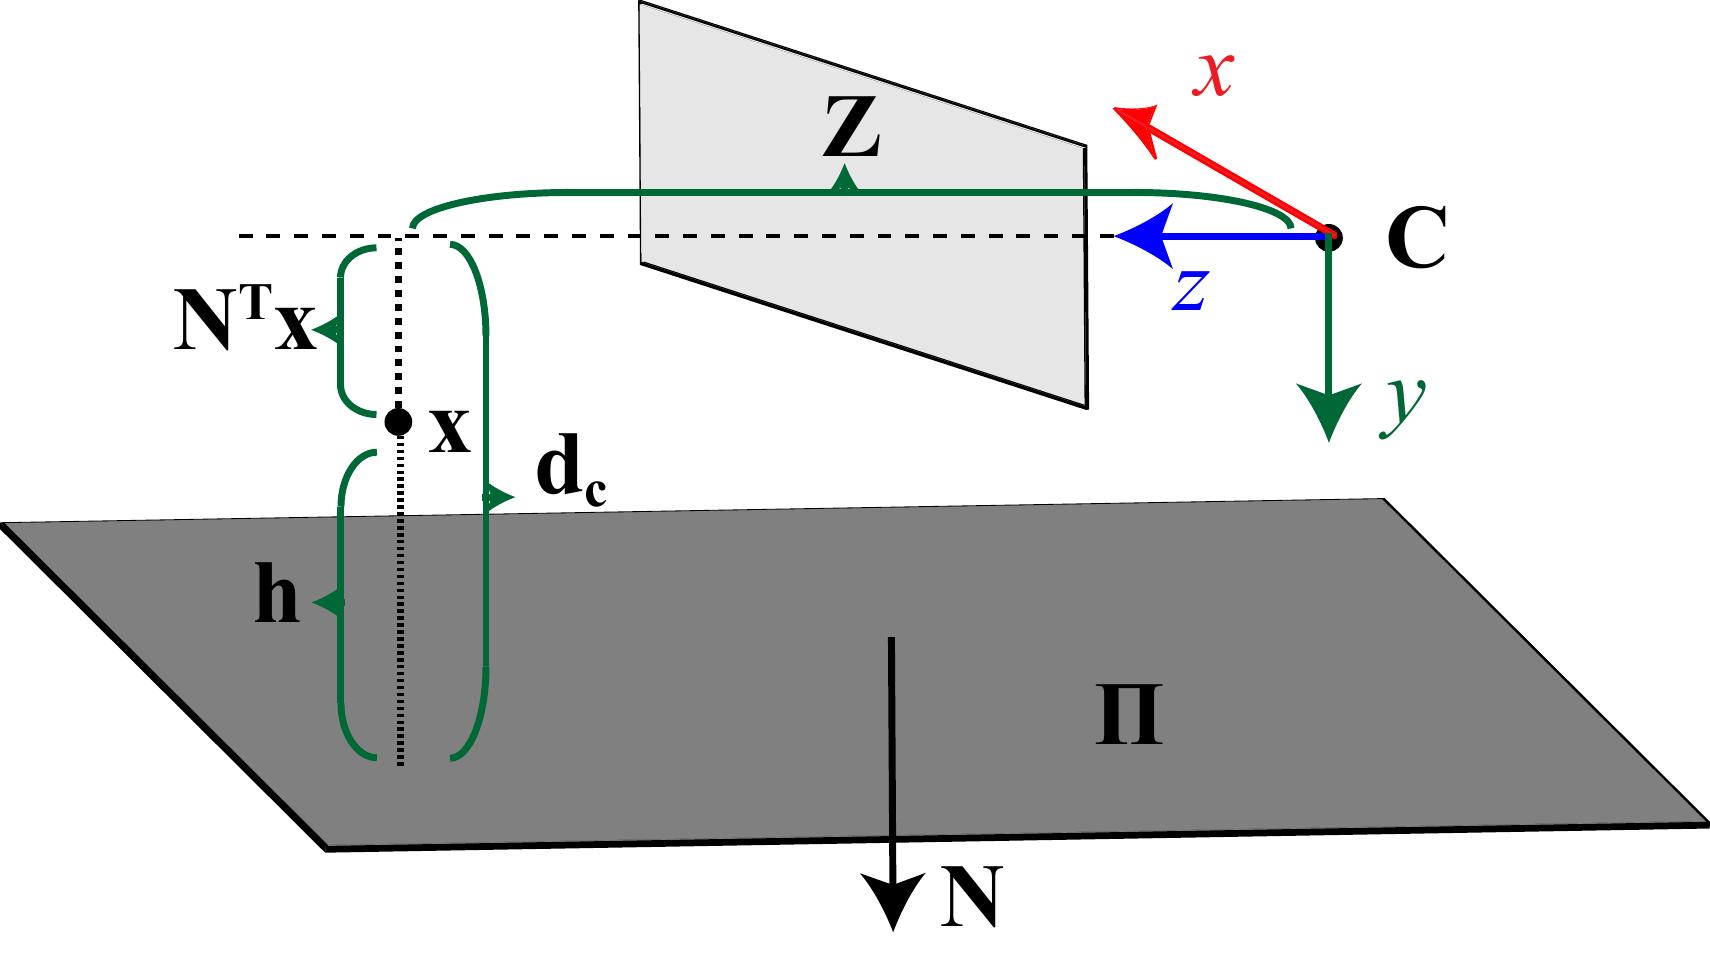}}
    \caption{\textbf{Visualization of the Planar Parallax.} \textit{Left:} The 3D point $\bx$ is projected to points $\bp$ and $\bp'$ on the target image $\bI_t$ and the source image $\bI_s$ respectively. Using the homography $\bH$ induced by the plane $\bPi$, the point $\bp'$ will be transformed to point $\bp_w$ on the target image. \textit{Right:} Calculating $\bh$, distance of $\bx$ to the $\bPi$ using the camera height $\bd_c$ and the normal vector $\bN$ of the plane. $\bC$ and $\bC'$ are the camera centers of $\bI_t$ and $\bI_s$ and $\bZ$ is the depth of the point.
    }
    \label{fig:pp}
    \vspace{-3.5pt}
\end{figure*}
