# Supplementary material for: DepthP+P: Metric Accurate Monocular Depth Estimation using Planar and Parallax
Source: arXiv:2301.02092 source file (2023-01-05)
Supplement: Supplementary file 4 [file qual2.tex]

\begin{figure*}[h]
    \def\hspacing{0.002\linewidth}
    \def\vspacing{0.03cm}
    \def\imgw{0.198\linewidth}
    \begin{tabular}{ccccc}
    \hspace{0.016\linewidth}Input Image &  \hspace{0.001\linewidth} Monodepth2 [10] &  \hspace{0.018\linewidth}DNet [32] &
    \hspace{0.035\linewidth} Ours-Mono & 
    \hspace{0.035\linewidth} Ours-Stereo\\
    \end{tabular}

\includegraphics[width=\imgw]{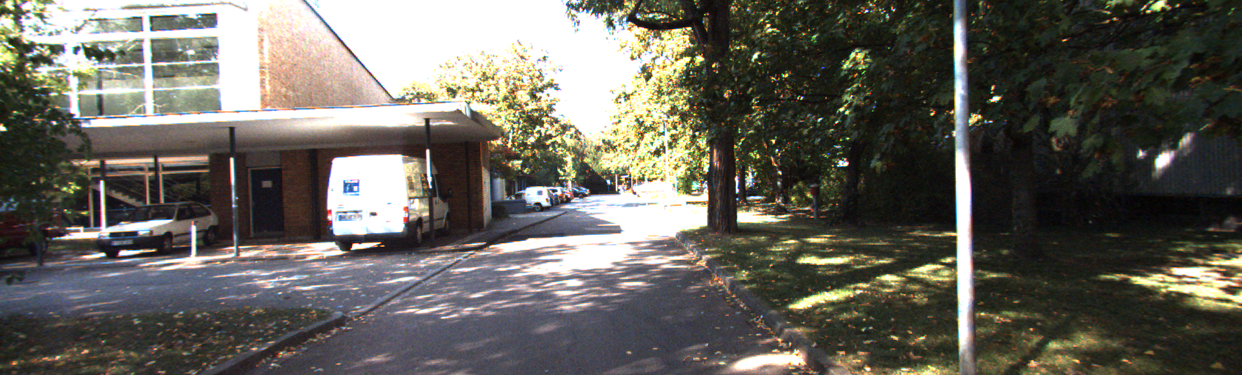}\hspace{\hspacing}%
    \includegraphics[width=\imgw]{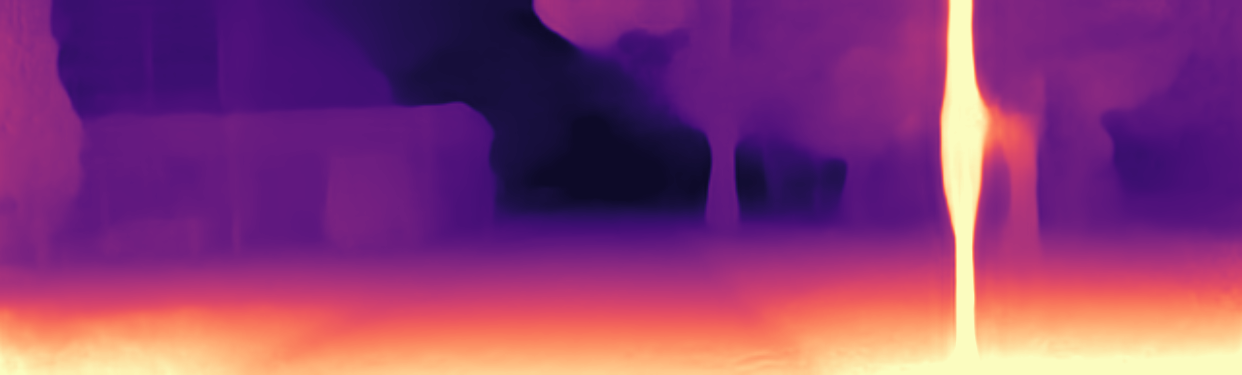}\hspace{\hspacing}%
    \includegraphics[width=\imgw]{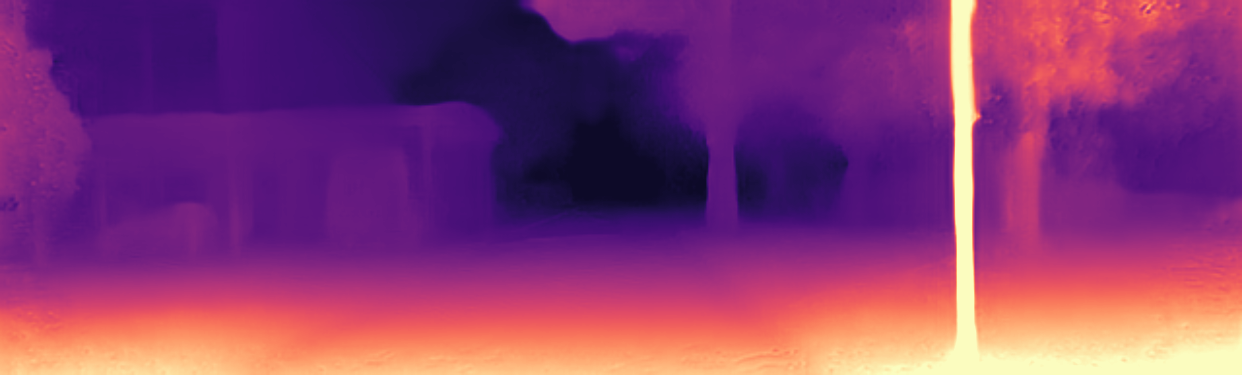}\hspace{\hspacing}%
    \includegraphics[width=\imgw]{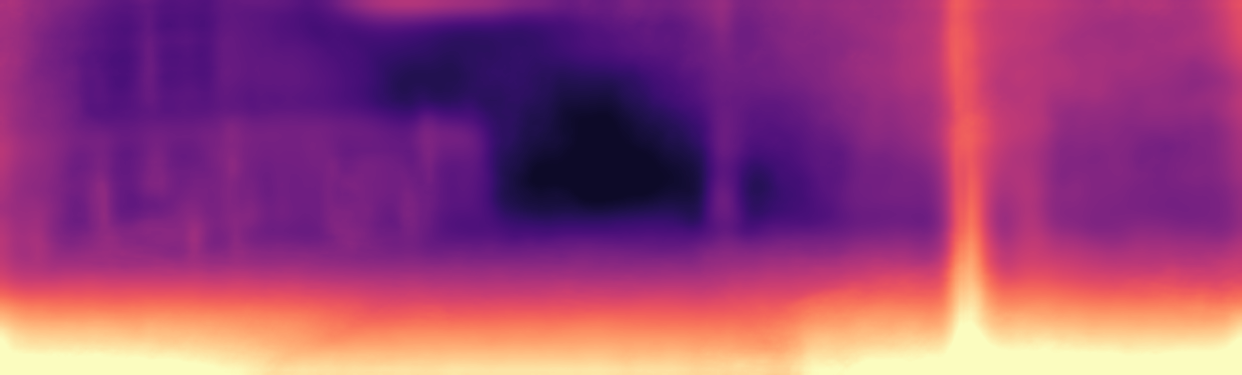}\hspace{\hspacing}%
    \includegraphics[width=\imgw]{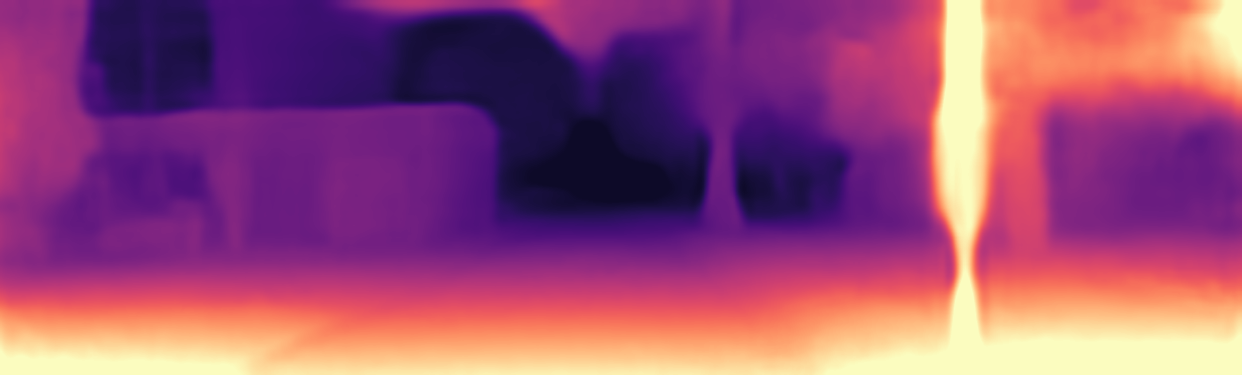}\hspace{\hspacing}%
    \vspace{\vspacing}

% \includegraphics[width=\imgw]{images/qual/0594.png}\hspace{\hspacing}%
%     \includegraphics[width=\imgw]{images/qual/0594_monodepth2.png}\hspace{\hspacing}%
%     \includegraphics[width=\imgw]{images/qual/0594_dnet.png}\hspace{\hspacing}%
%     \includegraphics[width=\imgw]{images/qual/0594_ours_mono.png}\hspace{\hspacing}%
%     \includegraphics[width=\imgw]{images/qual/0594_ours_stereo.png}\hspace{\hspacing}%
%     \vspace{\vspacing}

\includegraphics[width=\imgw]{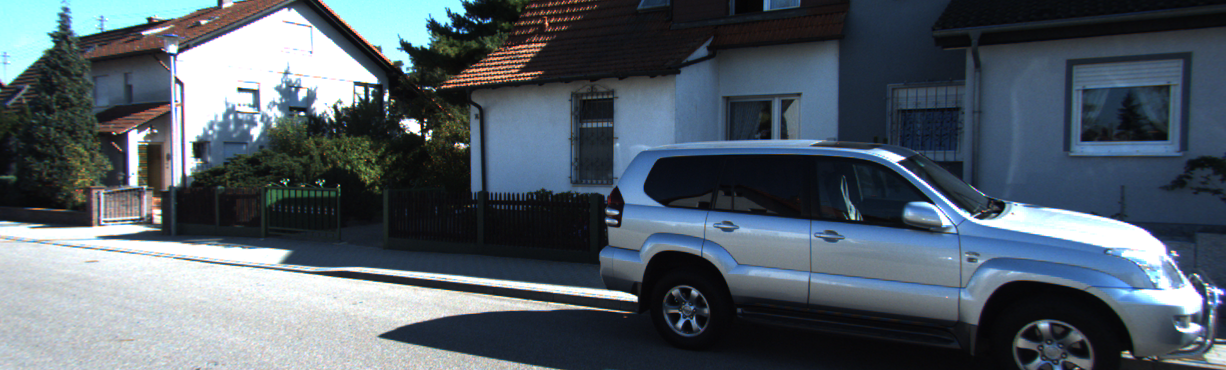}\hspace{\hspacing}%
    \includegraphics[width=\imgw]{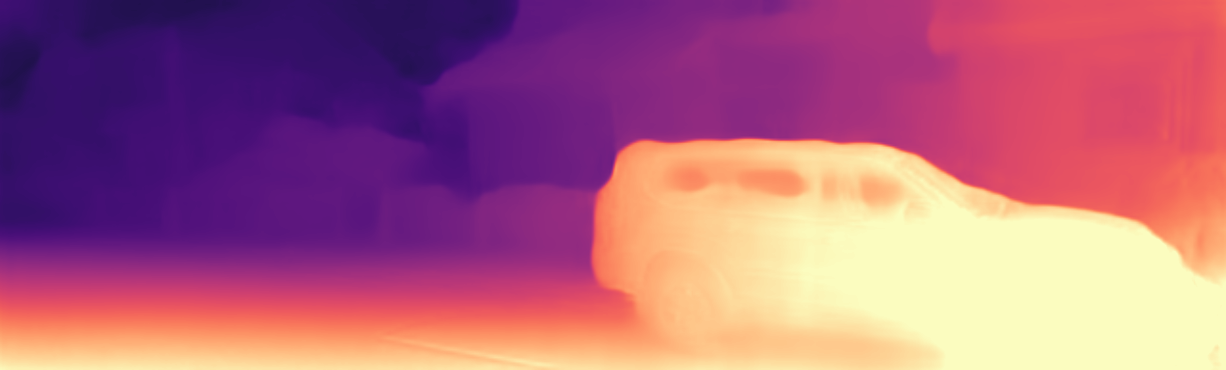}\hspace{\hspacing}%
    \includegraphics[width=\imgw]{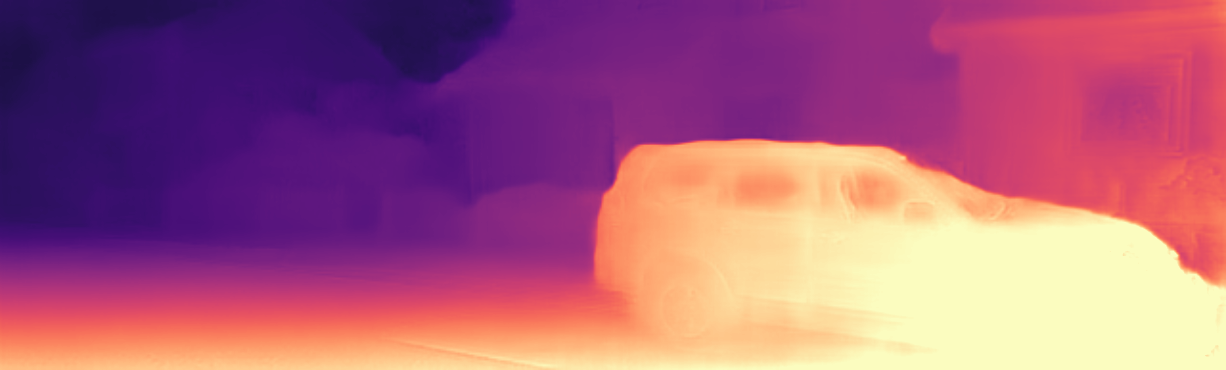}\hspace{\hspacing}%
    \includegraphics[width=\imgw]{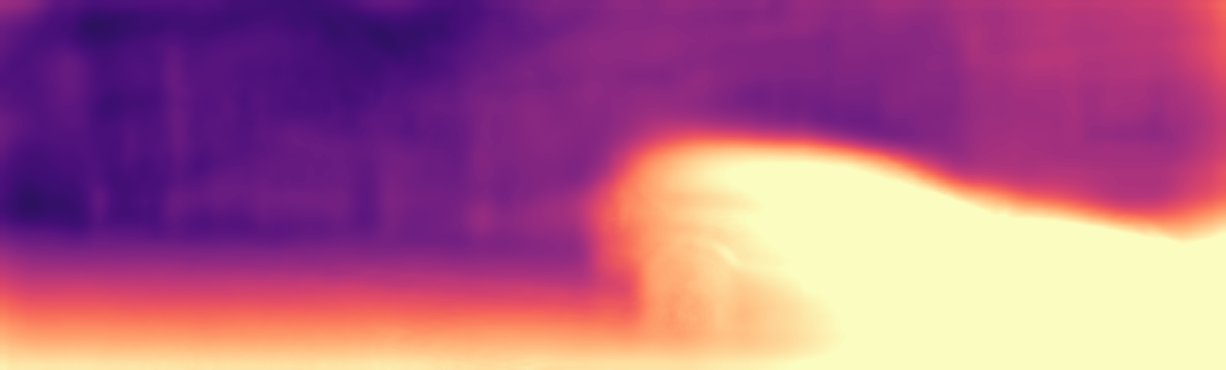}\hspace{\hspacing}%
    \includegraphics[width=\imgw]{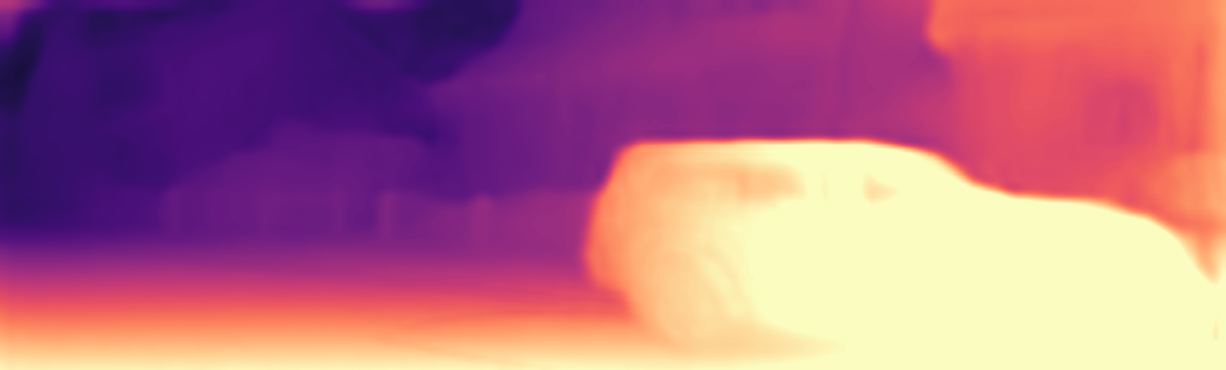}\hspace{\hspacing}%
    \vspace{\vspacing}

\includegraphics[width=\imgw]{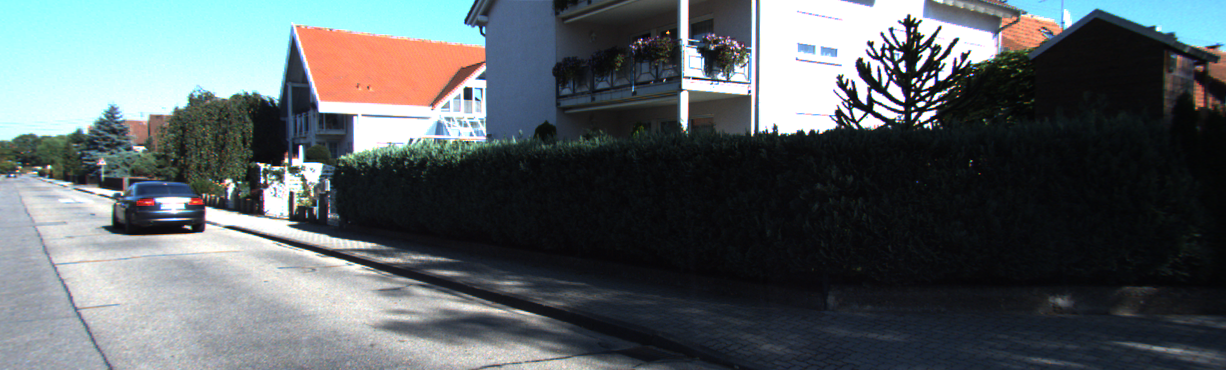}\hspace{\hspacing}%
    \includegraphics[width=\imgw]{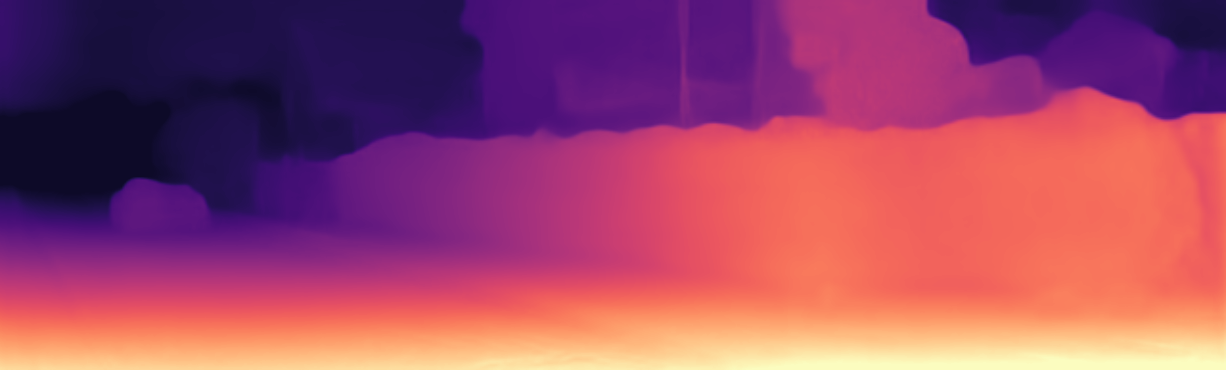}\hspace{\hspacing}%
    \includegraphics[width=\imgw]{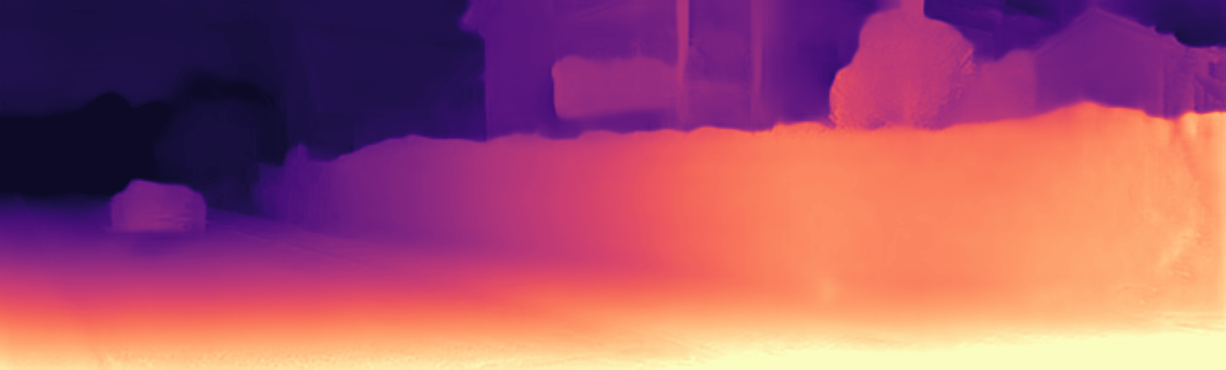}\hspace{\hspacing}%
    \includegraphics[width=\imgw]{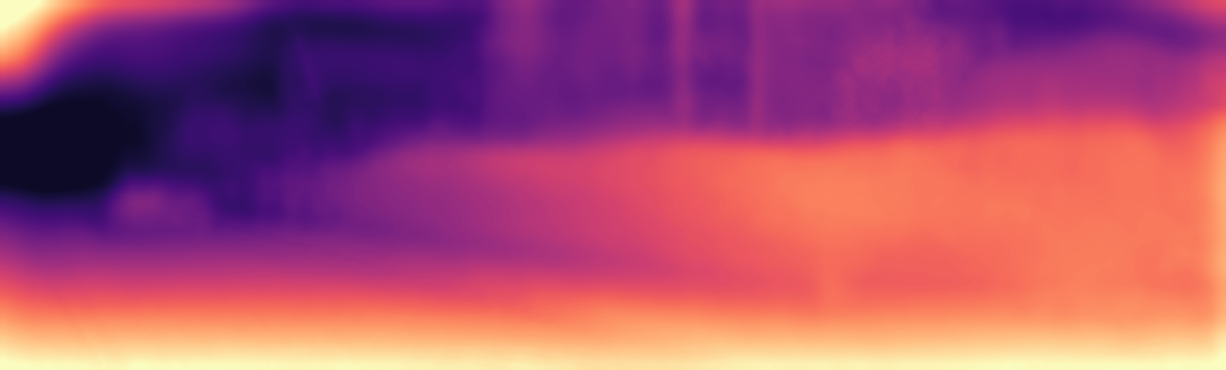}\hspace{\hspacing}%
    \includegraphics[width=\imgw]{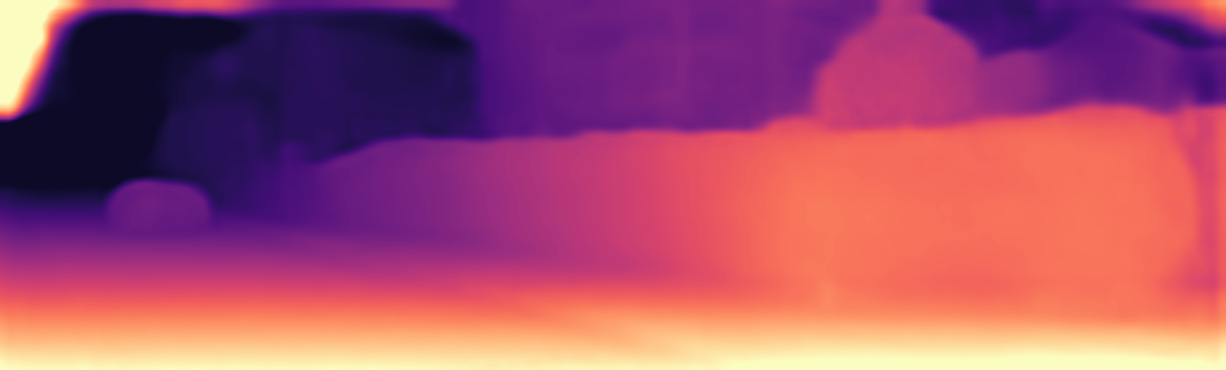}\hspace{\hspacing}%
    \vspace{\vspacing}

\includegraphics[width=\imgw]{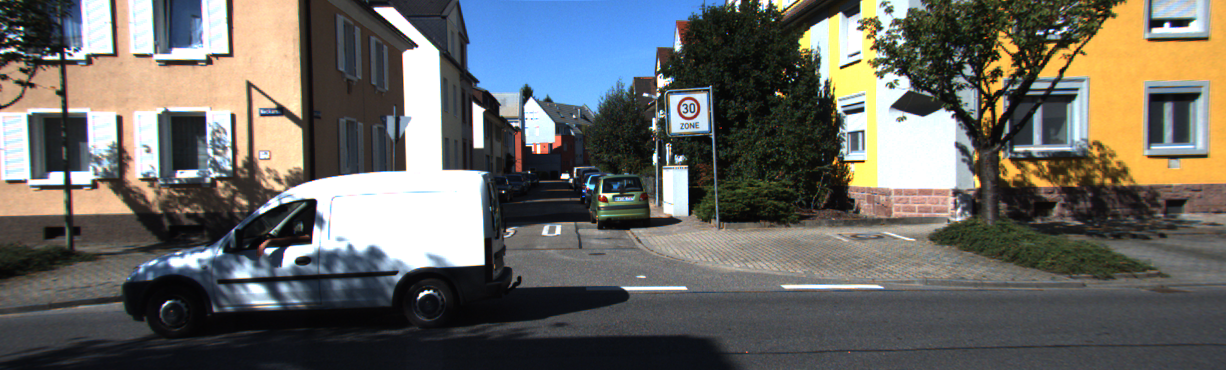}\hspace{\hspacing}%
    \includegraphics[width=\imgw]{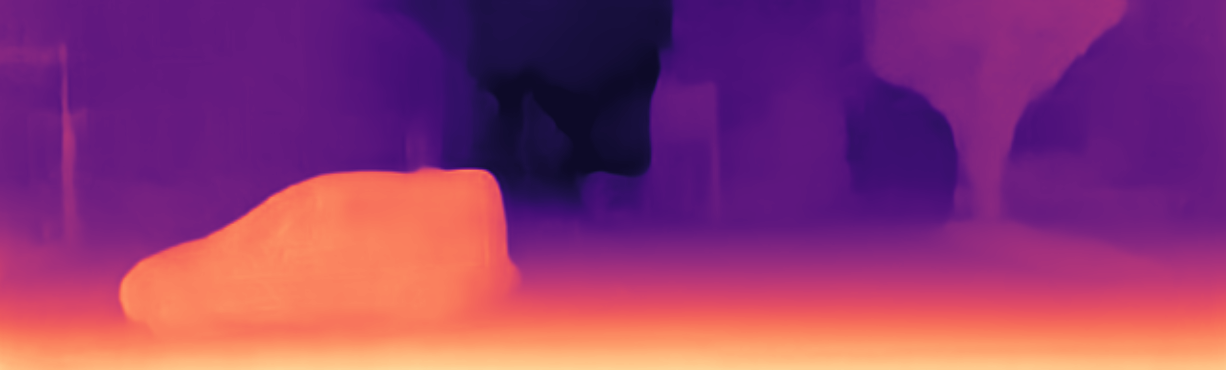}\hspace{\hspacing}%
    \includegraphics[width=\imgw]{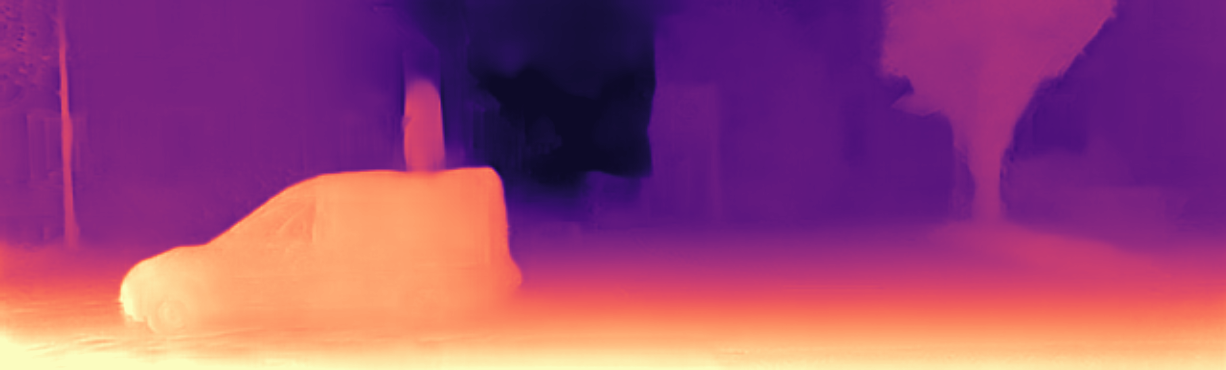}\hspace{\hspacing}%
    \includegraphics[width=\imgw]{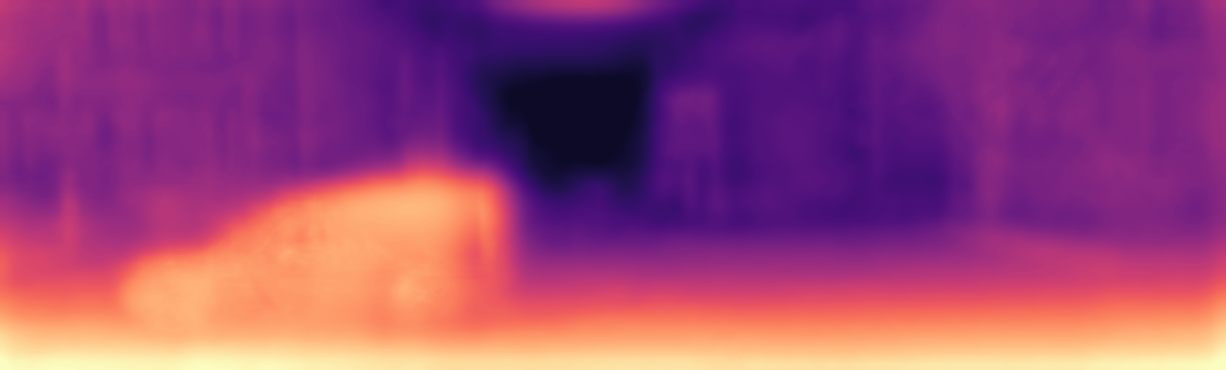}\hspace{\hspacing}%
    \includegraphics[width=\imgw]{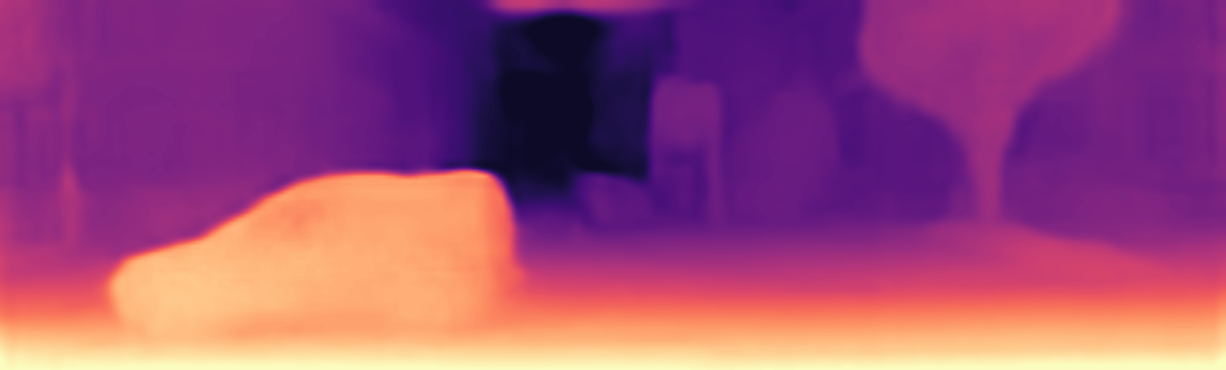}\hspace{\hspacing}%
    \vspace{\vspacing}

\includegraphics[width=\imgw]{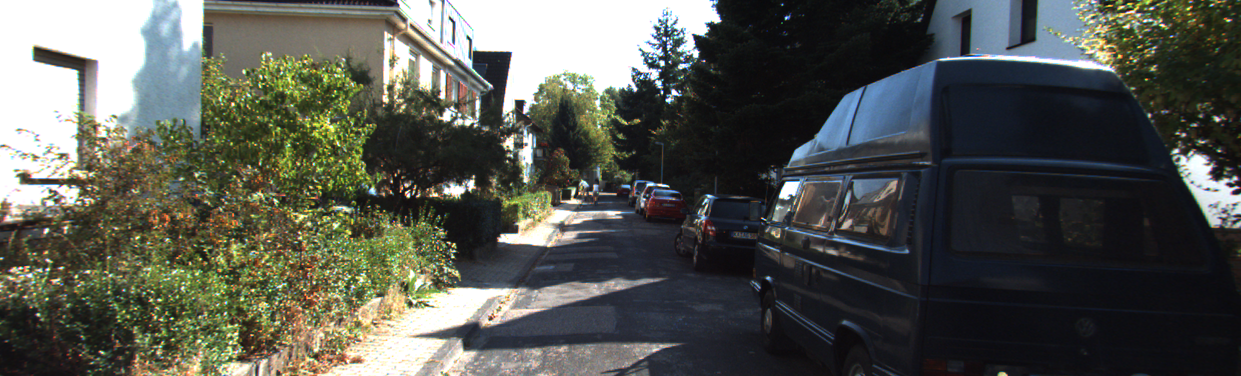}\hspace{\hspacing}%
    \includegraphics[width=\imgw]{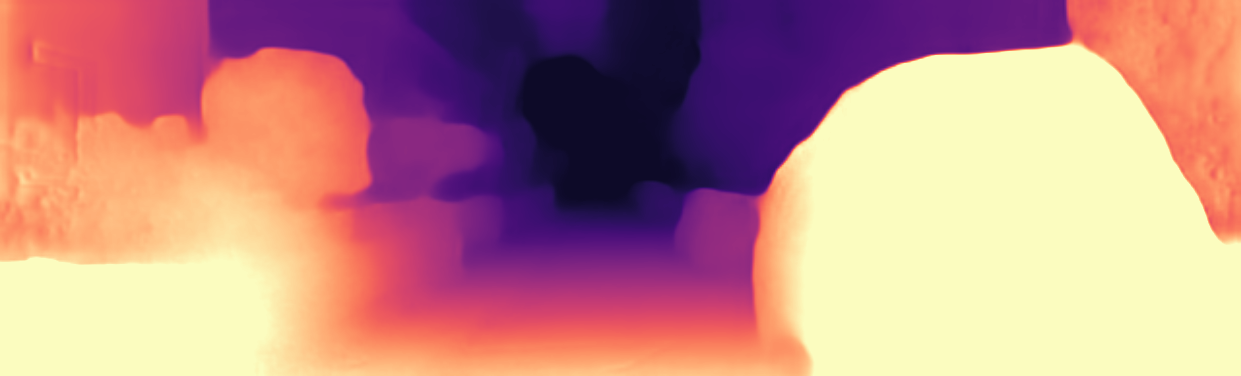}\hspace{\hspacing}%
    \includegraphics[width=\imgw]{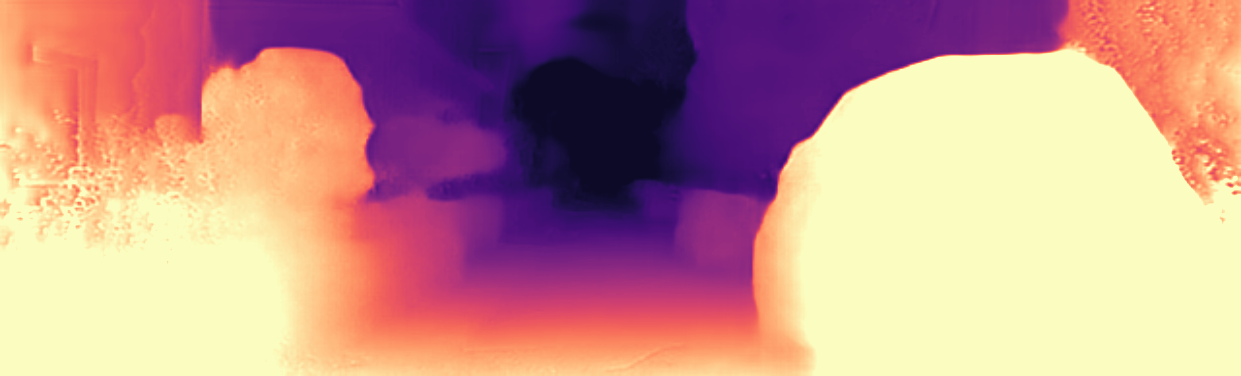}\hspace{\hspacing}%
    \includegraphics[width=\imgw]{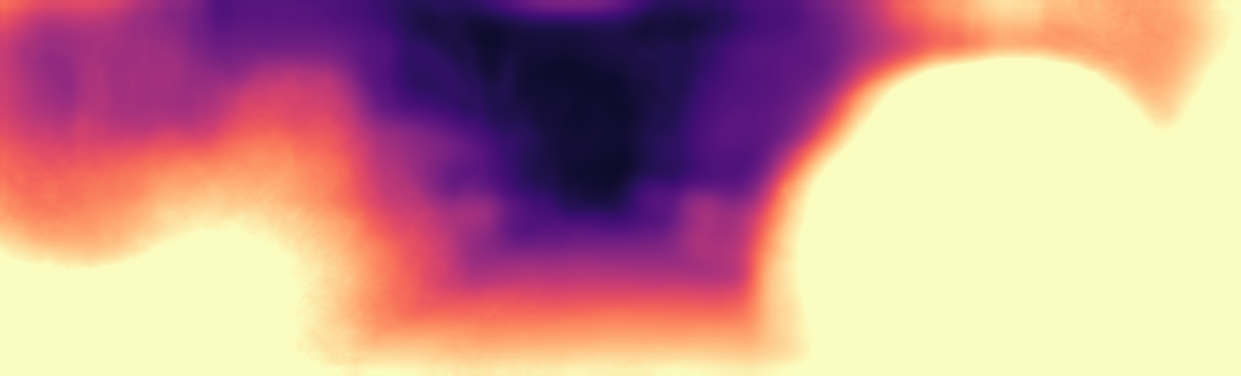}\hspace{\hspacing}%
    \includegraphics[width=\imgw]{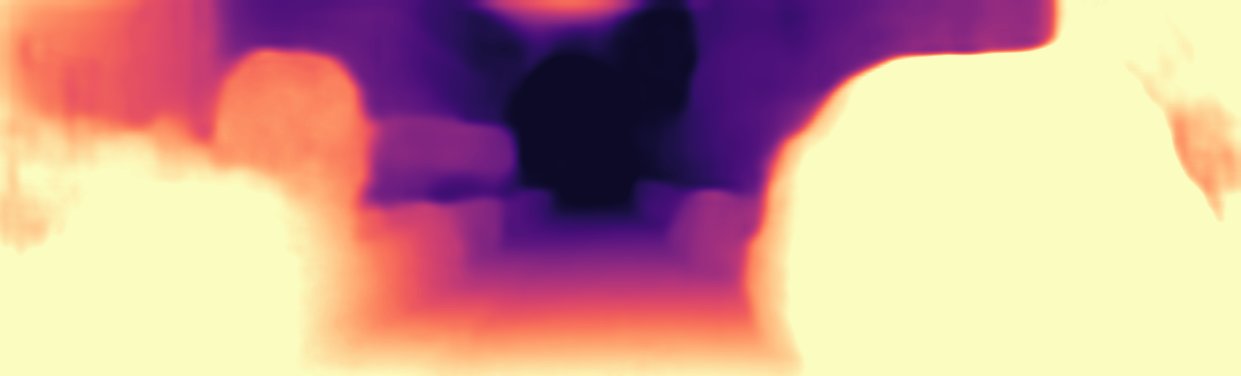}\hspace{\hspacing}%
    \vspace{\vspacing}

% \includegraphics[width=\imgw]{images/qual/0679.png}\hspace{\hspacing}%
%     \includegraphics[width=\imgw]{images/qual/0679_monodepth2.png}\hspace{\hspacing}%
%     \includegraphics[width=\imgw]{images/qual/0679_dnet.png}\hspace{\hspacing}%
%     \includegraphics[width=\imgw]{images/qual/0679_ours_mono.png}\hspace{\hspacing}%
%     \includegraphics[width=\imgw]{images/qual/0679_ours_stereo.png}\hspace{\hspacing}%
%     \vspace{\vspacing}

\includegraphics[width=\imgw]{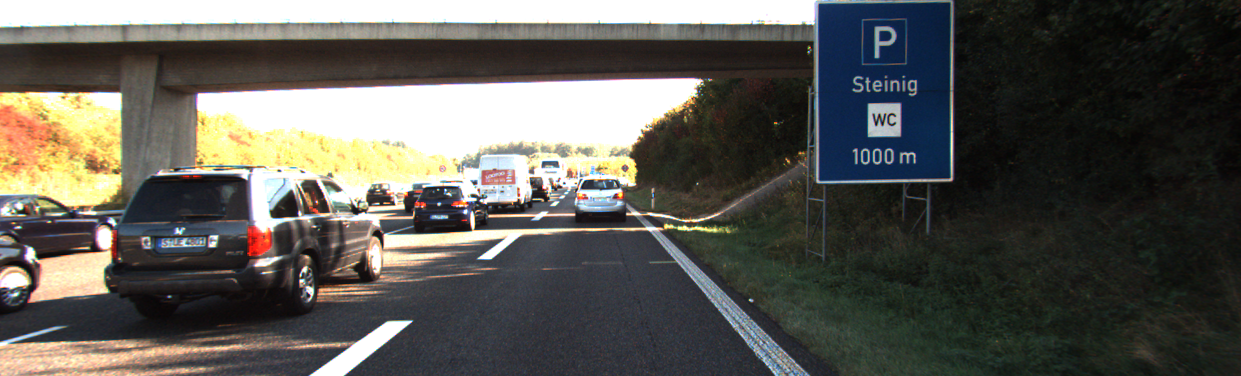}\hspace{\hspacing}%
    \includegraphics[width=\imgw]{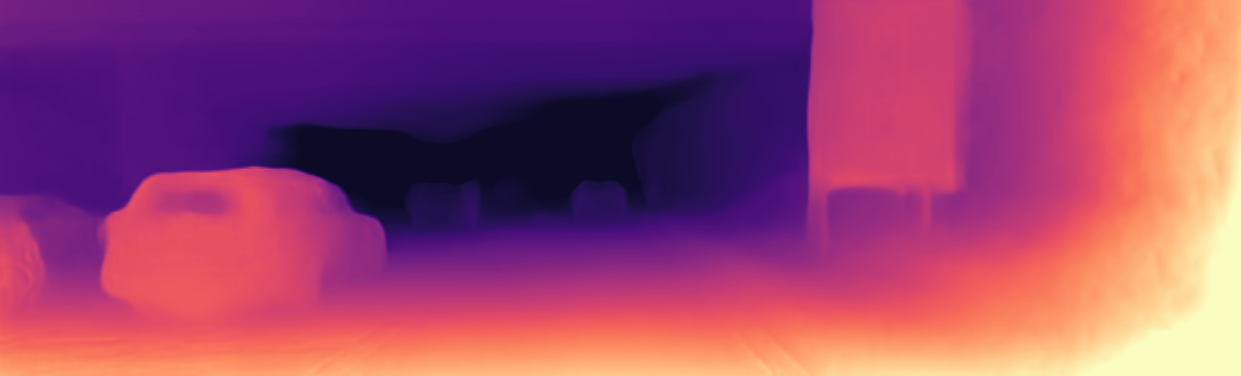}\hspace{\hspacing}%
    \includegraphics[width=\imgw]{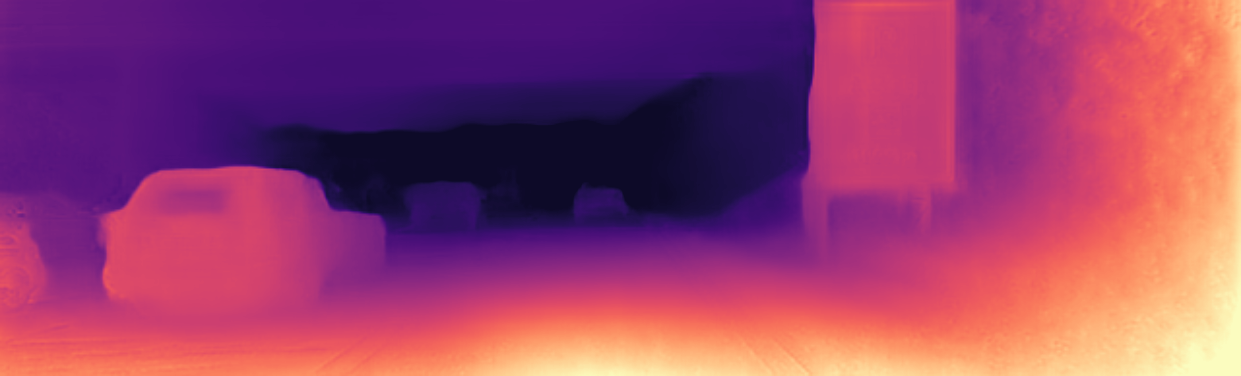}\hspace{\hspacing}%
    \includegraphics[width=\imgw]{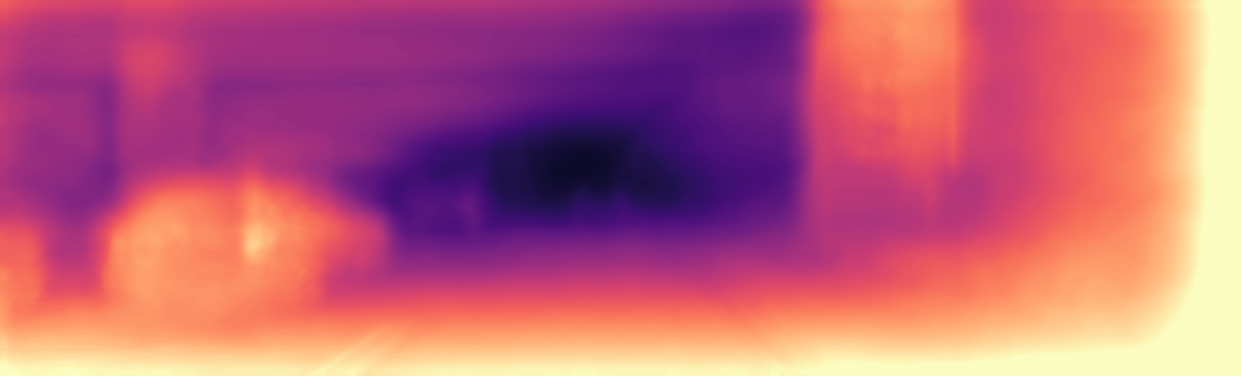}\hspace{\hspacing}%
    \includegraphics[width=\imgw]{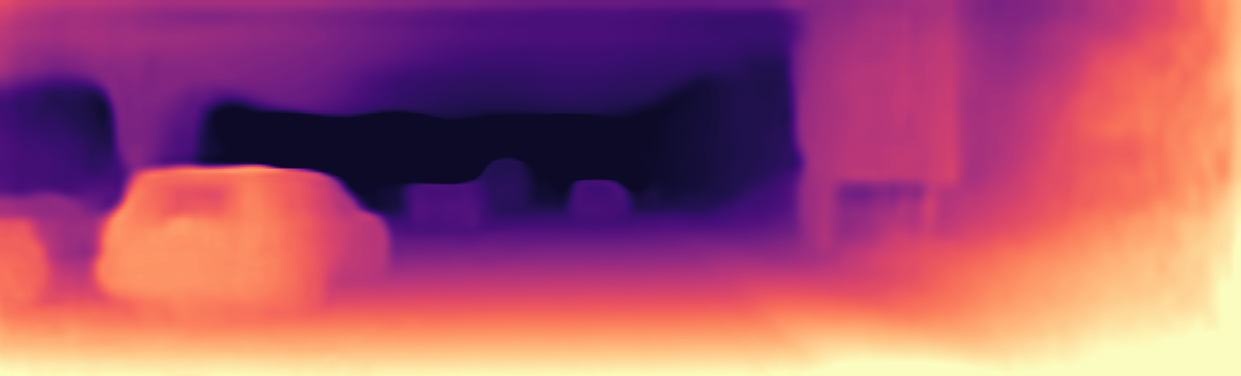}\hspace{\hspacing}%
    \vspace{\vspacing}

% \includegraphics[width=\imgw]{images/qual/0694.png}\hspace{\hspacing}%
%     \includegraphics[width=\imgw]{images/qual/0694_monodepth2.png}\hspace{\hspacing}%
%     \includegraphics[width=\imgw]{images/qual/0694_dnet.png}\hspace{\hspacing}%
%     \includegraphics[width=\imgw]{images/qual/0694_ours_mono.png}\hspace{\hspacing}%
%     \includegraphics[width=\imgw]{images/qual/0694_ours_stereo.png}\hspace{\hspacing}%
%     \vspace{\vspacing}

\includegraphics[width=\imgw]{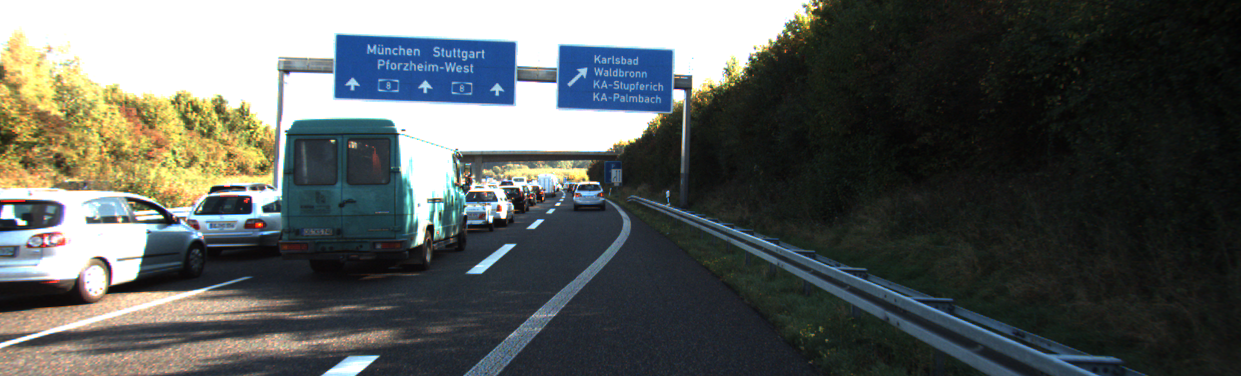}\hspace{\hspacing}%
    \includegraphics[width=\imgw]{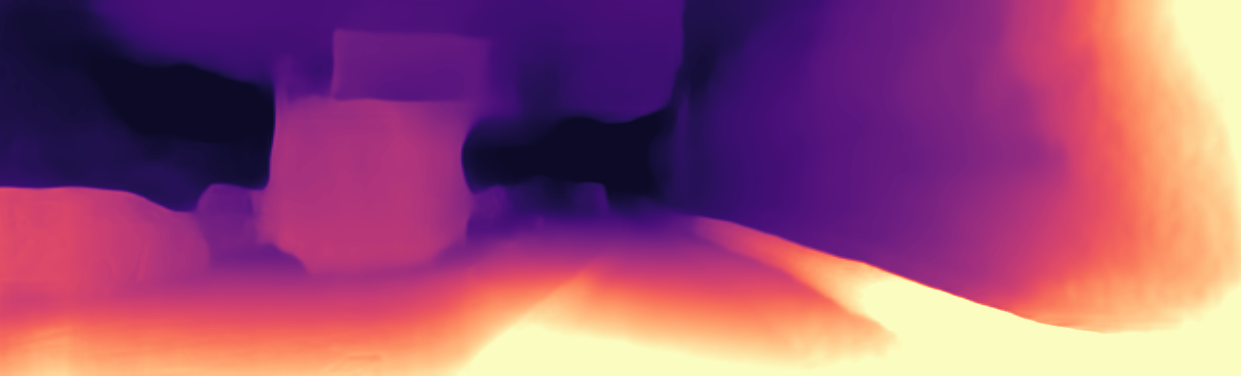}\hspace{\hspacing}%
    \includegraphics[width=\imgw]{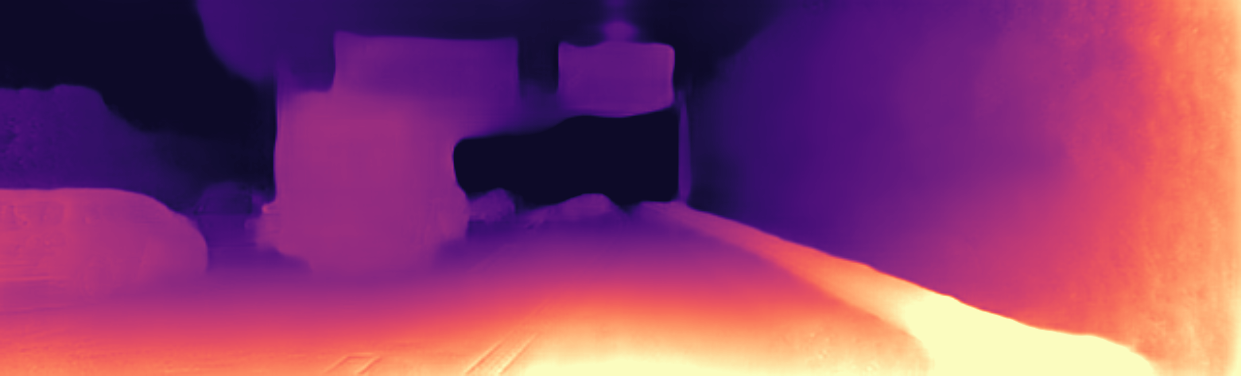}\hspace{\hspacing}%
    \includegraphics[width=\imgw]{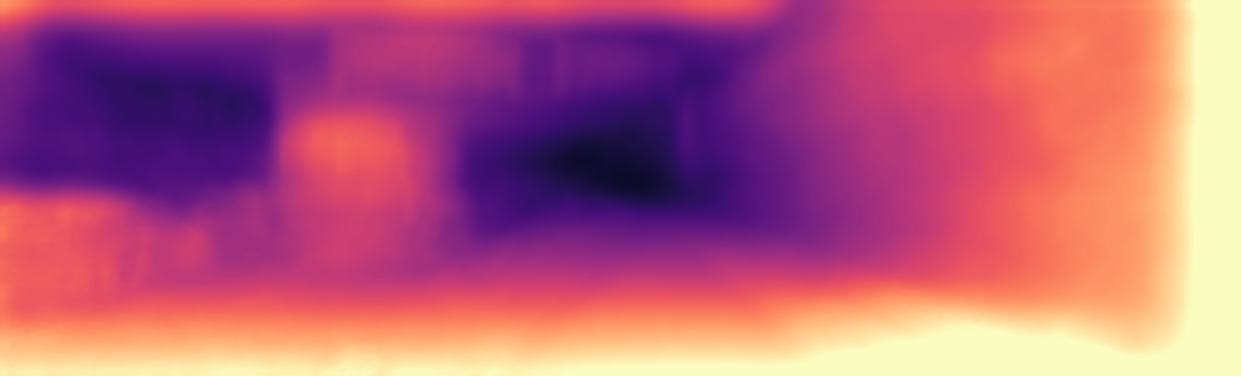}\hspace{\hspacing}%
    \includegraphics[width=\imgw]{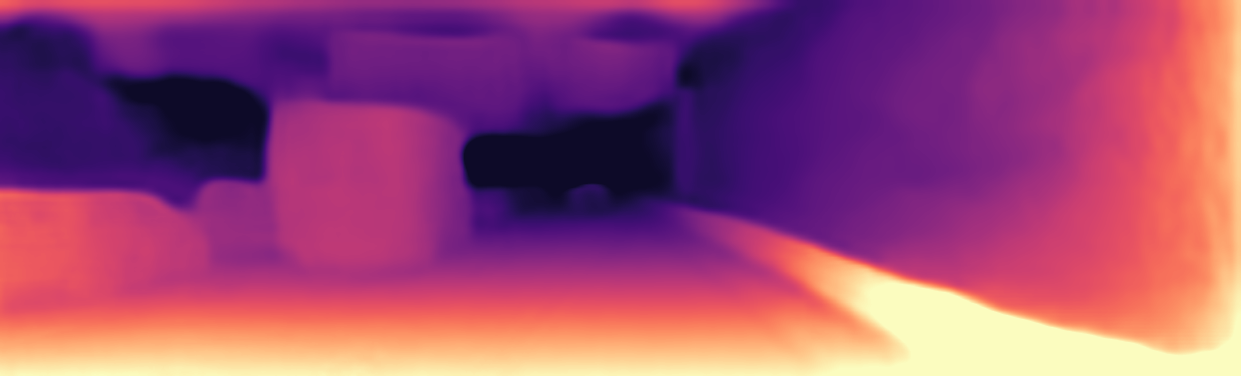}\hspace{\hspacing}%
    \vspace{\vspacing}

    \caption{{\bf Qualitative Results.}
    }
    \label{supp_fig:qualitative_results2}
    % \vspace{-3.5pt}
\end{figure*}
