# Supplementary material for: DepthP+P: Metric Accurate Monocular Depth Estimation using Planar and Parallax
Source: arXiv:2301.02092 source file (2023-01-05)
Supplement: Supplementary file 7 [file derivation_all.tex]

\section{Derivation}
\label{sec:derivation}
\begin{equation}
    \bx = \bR \bx'+\bt
\end{equation}

\begin{equation}
    \bh = \bd_c - \bN^T\bx'
\end{equation}

\begin{equation}
    1 = \frac{\bh + \bN^T\bx'}{\bd_c}  
\end{equation}

\begin{equation}
     \bx = \bR \bx'+\bt \left( \frac{\bh + \bN^T\bx'}{\bd_c}  \right)
\end{equation}

\begin{equation}
     \bx = \left( \bR + \frac{\bt\bN^T}{\bd_c} \right)\bx' + \frac{\bh}{\bd_c}\bt
\end{equation}

\begin{equation}
     \bZ \bK^{-1}\bp = \left( \bR + \frac{\bt\bN^T}{\bd_c} \right)\bZ' \bK'^{-1}\bp' + \frac{\bh}{\bd_c} \bt
\end{equation}

\begin{equation}
     \frac{\bZ}{\bZ'} \bp = \bK \left( \bR + \frac{\bt\bN^T}{\bd_c} \right) \bK'^{-1}\bp' + \frac{\bh}{\bZ' \bd_c} \bK \bt
\end{equation}

\begin{equation}
     \frac{\bZ}{\bZ'} \bp = \bH\bp' + \frac{\bh}{\bZ' \bd_c} \bK \bt
\end{equation}

\begin{equation}
     \frac{\bZ}{\bZ'}= \bH_3\bp' + \frac{\bh}{\bZ' \bd_c} \bK_3 \bt
\end{equation}

\begin{equation}
     \frac{\bZ}{\bZ'}= \bH_3\bp' + \frac{\bh}{\bZ' \bd_c} \bt_z
\end{equation}

\begin{equation}
     \bp = \frac{\bH\bp' + \frac{\bh}{\bZ' \bd_c} \bK \bt} {\bH_3\bp' + \frac{\bh}{\bZ' \bd_c} \bt_z}
\end{equation}

\begin{equation}
     \bp = \frac{\bH\bp'}{\bH_3\bp'} - \frac{\bH\bp'}{\bH_3\bp'} +  \frac{\bH\bp' + \frac{\bh}{\bZ' \bd_c} \bK \bt} {\bH_3\bp' + \frac{\bh}{\bZ' \bd_c} \bt_z}
\end{equation}

\begin{equation}
     \bp = \frac{\bH\bp'}{\bH_3\bp'} - \frac{\bH\bp' \left( \bH_3\bp' + \frac{\bh}{\bZ' \bd_c} \bt_z \right) }{\bH_3\bp' \left( \bH_3\bp' + \frac{\bh}{\bZ' \bd_c} \bt_z \right) } + \frac{\bH_3\bp' \left( \bH\bp' + \frac{\bh}{\bZ' \bd_c} \bK \bt \right)}{\bH_3\bp' \left( \bH_3\bp' + \frac{\bh}{\bZ' \bd_c} \bt_z \right) }
\end{equation}

\begin{equation}
     \bp = \frac{\bH\bp'}{\bH_3\bp'} - \frac{\bH\bp' \left( \frac{\bh}{\bZ' \bd_c} \bt_z \right) }{\bH_3\bp' \left( \bH_3\bp' + \frac{\bh}{\bZ' \bd_c} \bt_z \right) } + \frac{\bH_3\bp' \left(\frac{\bh}{\bZ' \bd_c} \bK \bt \right)}{\bH_3\bp' \left( \bH_3\bp' + \frac{\bh}{\bZ' \bd_c} \bt_z \right) }
\end{equation}

\begin{equation}
     \bp = \frac{\bH\bp'}{\bH_3\bp'} - \frac{\bH\bp' \left( \frac{\bh}{\bZ' \bd_c} \bt_z \right) }{\bH_3\bp' \left( \frac{\bZ}{\bZ'} \right) } + \frac{\bH_3\bp' \left(\frac{\bh}{\bZ' \bd_c} \bK \bt \right)}{\bH_3\bp' \left( \frac{\bZ}{\bZ'} \right) }
\end{equation}

\begin{equation}
     \bp = \frac{\bH\bp'}{\bH_3\bp'} - \frac{\bh \bt_z}{\bZ \bd_c}\frac{\bH\bp'}{\bH_3\bp'} + \frac{\bh}{\bZ \bd_c}\bK \bt 
\end{equation}

\begin{equation}
     \bp = \bp_w - \frac{\bh \bt_z}{\bZ \bd_c}\bp_w + \frac{\bh}{\bZ \bd_c}\bK \bt 
\end{equation}

\begin{equation}
     \bp - \frac{\bh \bt_z}{\bZ \bd_c}\bp = \bp_w - \frac{\bh \bt_z}{\bZ \bd_c}\bp_w + \frac{\bh}{\bZ \bd_c}\bK \bt - \frac{\bh \bt_z}{\bZ \bd_c}\bp
\end{equation}

\begin{equation}
     \bp \left(1- \frac{\bh \bt_z}{\bZ \bd_c}\right) = \bp_w \left(1- \frac{\bh \bt_z}{\bZ \bd_c}\right) + \frac{\bh}{\bZ \bd_c}\bK \bt   - \frac{\bh \bt_z}{\bZ \bd_c}\bp
\end{equation}

\begin{equation}
     \bp  = \bp_w  + \frac{\frac{\bh}{\bZ \bd_c}\bK \bt   - \frac{\bh \bt_z}{\bZ \bd_c}\bp}{1- \frac{\bh \bt_z}{\bZ \bd_c}} 
\end{equation}

\begin{equation}
     \bp_w - \bp = \frac{\frac{\bh \bt_z}{\bZ \bd_c}\bp - \frac{\bh}{\bZ \bd_c}\bK \bt   }{1- \frac{\bh \bt_z}{\bZ \bd_c}} 
\end{equation}

\begin{equation}
     \bp_w - \bp = \frac{\frac{\bh \bt_z}{\bZ}\bp - \frac{\bh}{\bZ}\bK \bt   }{\bd_c- \frac{\bh \bt_z}{\bZ}} 
\end{equation}

\begin{equation}
     \bp_w - \bp = \frac{\gamma\bt_z\bp - \gamma\bK \bt   }{\bd_c- \gamma\bt_z} 
\end{equation}

\begin{equation}
     \bp_w - \bp = \frac{\gamma}{\bd_c- \gamma\bt_z} \left( \bt_z\bp - \gamma\bK \bt   \right)
\end{equation}
