# Supplementary material for: DepthP+P: Metric Accurate Monocular Depth Estimation using Planar and Parallax
Source: arXiv:2301.02092 source file (2023-01-05)
Supplement: Supplementary file 13 [file kitti_main_2.tex]

\begin{table*}[t]
    \centering
    \begin{tabular}{l | l| c c c c | c c c }
    \toprule
{\multirow{2}{*}{\bf GT}} & {\multirow{2}{*}{\bf Method}} & \multicolumn{4}{c}{Lower Better} & \multicolumn{3}{c}{Higher Better} \tabularnewline 
& & Abs Rel & Sq Rel & RMSE & RMSE$_{log}$ & $\delta < 1.25$ & $\delta < 1.25^2$ & $\delta < 1.25^3$\tabularnewline \hline
\parbox[t]{0.2mm}{\multirow{16}{*}{\rotatebox[origin=c]{90}{\small{Original Ground Truth \cite{Eigen2014NeurIPS}}}}}
& Zhou \etal \cite{Zhou2017CVPR} &  0.183 & 1.595 & 6.709 & 0.270 & 0.734 & 0.902 & 0.959 \tabularnewline 
& Yang \etal \cite{Yang2018AAAI} &  0.182 & 1.481 & 6.501 & 0.267 & 0.725 & 0.906 & 0.963 \tabularnewline 
& Mahjourian \etal \cite{Mahjourian2018CVPR} &  0.163 & 1.240 & 6.220 & 0.250 & 0.762 & 0.916 & 0.968 \tabularnewline
& Yin \etal \cite{Yin2018CVPR} &  0.149 & 1.060 & 5.567 & 2.226 & 0.796 & 0.935 & 0.975 \tabularnewline
& Wang \etal \cite{Wang2018CVPR} &  0.151 & 1.257 & 5.583 & 0.228 & 0.810 & 0.936 & 0.974 \tabularnewline
& Zou \etal \cite{Zou2018ECCV} &  0.150 & 1.124 & 5.507 & 0.223 & 0.806 & 0.933 & 0.973 \tabularnewline
& Yang \etal \cite{Yang2018CVPR} &  0.162 & 1.352 & 6.276 & 0.252 & - & - & - \tabularnewline
& Ranjan \etal \cite{Ranjan2019CVPR} &  0.148 & 1.149 & 5.464 & 0.226 & 0.815 & 0.935 & 0.973 \tabularnewline
& Luo \etal \cite{Luo2019PAMI} &  0.141 & 1.029 & 5.350 & 0.216 & 0.816 & 0.941 & 0.976 \tabularnewline
& Chen \etal \cite{Chen2019ICCV} &  0.118 & 0.905 & 5.096 & 0.211 & 0.839 & 0.945 & 0.977 \tabularnewline
& Godard \etal \cite{Godard2019ICCV} &  \textbf{0.110} & 0.831 & \underline{4.642} & \textbf{0.187} & \textbf{0.883} & \textbf{0.962} & \textbf{0.982} \tabularnewline
& Guizilini \etal \cite{Guizilini2020CVPR} &  \underline{0.111} & \textbf{0.785}   & \textbf{4.601} & \underline{0.189} & 0.878 & \underline{0.960} & \textbf{0.982}\tabularnewline 
& Safadoust \etal &  \textbf{0.110} & \underline{0.792} & 4.700 & \underline{0.189} & \underline{0.881} & \underline{0.960} & \textbf{0.982} \tabularnewline
& DepthP+P (Ours) &  0.152 & 1.322 & 6.185 & 0.239 & 0.781 & 0.920 & 0.970 \tabularnewline \cline{2-9}
& Casser \etal \cite{Casser2019AAAI} & 0.141 & 1.026 & 5.291 & 0.215 & 0.816 & 0.945 & 0.979 \tabularnewline
& Guizilini \etal \cite{Guizilini2020CVPR} &  0.111 & 0.829 & 4.788 & 0.199 & 0.864 & 0.954 & 0.980 \tabularnewline
& Guizilini \etal \cite{Guizilini2020ICLR} & 0.102 & 0.698 & 4.381 & 0.178 & 0.896 & 0.964 & 0.984 \tabularnewline \hline\hline 
%\midrule
\parbox[t]{2mm}{\multirow{10}{*}{\rotatebox[origin=c]{90}{\small{Improved GT \cite{Uhrig2017THREEDV}}}}} %&
& Zhou \etal \cite{Zhou2017CVPR} &  0.176 & 1.532 & 6.129 & 0.244 & 0.758 & 0.921 & 0.971 \tabularnewline
& Mahjourian \etal \cite{Mahjourian2018CVPR} &  0.134 & 0.983 & 5.501 & 0.203 & 0.827 & 0.944 & 0.981 \tabularnewline
& Yin \etal \cite{Yin2018CVPR} &  0.132 & 0.994 & 5.240 & 0.193 & 0.833 & 0.953 & 0.985 \tabularnewline
& Wang \etal \cite{Wang2018CVPR} &  0.126 & 0.866 & 4.932 & 0.185 & 0.851 & 0.958 & 0.986 \tabularnewline
& Ranjan \etal \cite{Ranjan2019CVPR} &  0.123 & 0.881 & 4.834 & 0.181 & 0.860 & 0.959 & 0.985 \tabularnewline
& Luo \etal \cite{Luo2019PAMI} &  0.120 & 0.789 & 4.755 & 0.177 & 0.856 & 0.961 & 0.987 \tabularnewline
& Godard \etal \cite{Godard2019ICCV} &  \underline{0.085} & 0.468 & \underline{3.672} & \underline{0.128} & \underline{0.921} & \underline{0.985} & \underline{0.995} \tabularnewline
& Guizilini \etal \cite{Guizilini2020CVPR} &  \textbf{0.078} & \textbf{0.420} & \textbf{3.485} & \textbf{0.121} & \textbf{0.931} & \textbf{0.986} & \textbf{0.996} \tabularnewline
& Safadoust \etal  &  \underline{0.085} & \underline{0.458} & 3.779 & 0.131 & 0.919 & \underline{0.985} & \textbf{0.996} \tabularnewline
& DepthP+P (Ours) &  0.134 & 1.042 & 5.566 & 0.199 & 0.820 & 0.946 & 0.983
\end{tabular}

    % \vspace{2pt}
    \caption{\textbf{Quantitative Results for Monocular Training on KITTI.} This table compares our proposed approaches, \textbf{MonoDepthSeg} and \textbf{DepthP+P}, to previous approaches on the KITTI dataset using the original and improved ground truth. 
    %dataset for depth estimations up to 80m. 
    The \textbf{Supervision} column shows different types of supervision used by different methods and \textbf{M} stands for monocular sequences. \textbf{Sem} and \textbf{Ins} refer to using semantic or instance information, respectively. \textbf{v} refers to velocity supervision. We show the results for the input resolution $640 \times 192$. The best self-supervised method in each column is shown in bold and the second best is underlined.}
    \label{tab:kitti_main2}
    % \vspace{-2pt}
\end{table*}
